# Supplementary material for: Flux and storage of energy in non-equilibrium, stationary states
Source: arXiv:1902.10013 ancillary file (2019-02-26)
Supplement: Supplementary file 1 [file SM-holyst.pdf]

# Supplementary Material:

# Flux and storage of energy in non-equilibrium, stationary states.

Robert Hołyst, Anna Maciołek, Yirui Zhang, Marek Litniewski, Piotr Knychała, Maciej Kasprzak, Michał Banaszak

*Ideal gas between two planar walls*:

Following the same reasoning as for the case (i), we calculate the energy density for the case of the external flux proportional to temperature (ii). We find $\tilde{T}(\tilde{z}) = \cos\left(\sqrt{\tilde{\lambda}_2}\tilde{z}\right)/\cos\sqrt{\tilde{\lambda}_2}$ and

$$\varepsilon(\tilde{\lambda}_2) = \frac{2\sqrt{\tilde{\lambda}_2}}{\cos(\sqrt{\tilde{\lambda}_2})\ln\left((1+\sin\sqrt{\tilde{\lambda}_2})/(1-\sin\sqrt{\tilde{\lambda}_2})\right)}. \tag{1}$$

We note that the above solution is valid for $0 < \sqrt{\tilde{\lambda}_2} < \pi/2$. For larger values of $\tilde{\lambda}_2$, the system is not able to sustain the stationary state.

For the ratio of the energy storage $\Delta U = U - U_0$ to the total energy flux $J_U$ in the unconstrained system we find

$$\frac{\Delta U}{J_U} = \frac{\varepsilon_0}{\lambda_2 T_0}\left[\frac{2\tilde{\lambda}_2}{\sin(\sqrt{\tilde{\lambda}_2})\ln\left(\frac{1+\sin\sqrt{\tilde{\lambda}_2}}{1-\sin\sqrt{\tilde{\lambda}_2}}\right)} - \frac{\sqrt{\tilde{\lambda}_2}}{\tan\sqrt{\tilde{\lambda}_2}}\right] \tag{2}$$

whereas the same ratio for the partitioned system is

$$\frac{U_1 + U_2 - U_0}{J_{U_1} + J_{U_2}} = \frac{\varepsilon_0}{\lambda_2 T_0}\left[g_1(\tilde{z}_1) + g_2(\tilde{z}_1) - \frac{2\sqrt{\tilde{\lambda}_2}}{\left(\tan\sqrt{\Lambda_-^{(2)}} + \tan\sqrt{\Lambda_+^{(2)}}\right)}\right], \tag{3}$$

with

$$g_1(\tilde{z}_1) = \frac{1}{\left(\tan\sqrt{\Lambda_-^{(2)}} + \tan\sqrt{\Lambda_+^{(2)}}\right)}\frac{\sqrt{\Lambda_-^{(2)}}}{\cos\sqrt{\Lambda_-^{(2)}}\ln\left(\frac{\cos\sqrt{\Lambda_-^{(2)}}}{1-\sin\sqrt{\Lambda_-^{(2)}}}\right)} \tag{4}$$

and

$$g_2(\tilde{z}_1) = \frac{1}{\left(\tan\sqrt{\Lambda_-^{(2)}} + \tan\sqrt{\Lambda_+^{(2)}}\right)}\frac{\sqrt{\Lambda_+^{(2)}}}{\cos\sqrt{\Lambda_+^{(2)}}\ln\left(\frac{1+\sin\sqrt{\Lambda_+^{(2)}}}{\cos\sqrt{\Lambda_+^{(2)}}}\right)} \tag{5}$$

where $\Lambda_-^{(2)} = \tilde{\lambda}_2(1-\tilde{z}_1)^2$ and $\Lambda_+^{(2)} = \tilde{\lambda}_2(1+\tilde{z}_1)^2$.

In order to solve the equation for the temperature distribution in the stationary state (Eq. 1 in the main article text) for the case (iii) of the density dependent external flux, we use relation $\tilde{\rho}(z) = \tilde{\varepsilon}/\tilde{T}(z)$ for an ideal gas and obtain $\tilde{T}(\tilde{z}) = \tilde{T}(0)\exp\Big(-\Big[\mathrm{erf}^{-1}\Big(\frac{\tilde{\lambda}_3\tilde{z}}{\tilde{T}(0)\sqrt{\pi\ln\tilde{T}(0)}}\Big)\Big]^2\Big)$, where $\tilde{T}(0)$ is a real solution of the implicit equation $\mathrm{erf}\Big(\sqrt{\ln\tilde{T}(0)}\Big) = \tilde{\lambda}_3 \mathrm{e}^{-\ln\tilde{T}(0)}/\Big(\sqrt{\pi\ln\tilde{T}(0)}\Big)$. The symmetry of the temperature profile about $z = 0$ dictates that the energy density is related to $\tilde{T}(0)$ via

$$\tilde{\varepsilon}(\tilde{\lambda}_3) = \frac{\tilde{\lambda}_3}{2}\frac{1}{\ln\tilde{T}(0)}. \tag{6}$$

Finally, in the case (iii) we have

$$\frac{\Delta U}{J_U} = \frac{\varepsilon_0}{\lambda_3\rho_0}\left(\frac{\tilde{\lambda}_3}{2\ln\tilde{T}(0)} - 1\right), \tag{7}$$

and

$$\frac{U_1 + U_2 - U_0}{J_{U_1} + J_{U_2}} = \frac{\varepsilon_0}{\lambda_3\rho_0}\left(\frac{(1-\tilde{z}_1)^3\tilde{\lambda}_3}{4\ln\tilde{T}(-\tilde{z}_1)} + \frac{(1+\tilde{z}_1)^3\tilde{\lambda}_3}{4\ln\tilde{T}(-\tilde{z}_1)} - 1\right). \tag{8}$$

Direct inspection for both cases (ii) and (iii) show that for fixed $\tilde{\lambda}_i > 0, i = 2, 3$ the inequality

$$\frac{\Delta U_1 + \Delta U_2}{J_{U_1} + J_{U_2}} \geq \frac{\Delta U}{J_U}. \tag{9}$$

holds in the range $0 \leq \tilde{z}_1 < 1$.

One can take into account that the thermal conductivity $\kappa$ for an ideal gas depends on temperature. The kinetic theory predicts [1]

$$\kappa = \frac{mC_V}{3\sqrt{2}\sigma}\langle v\rangle, \tag{10}$$

where $m$ is the mass of the particle, $C_V$ is the heat capacity, $\sigma$ is the collision cross section and $\langle v\rangle = \sqrt{8T/\pi m}$ is the averaged velocity. To simplify, we collect all constants into $c = 2C_V\sqrt{m/\pi}/3$ and $\kappa = c\sqrt{T}$. Then, Eq. 1 in the main text becomes

$$\frac{\partial}{\partial z}(\sqrt{T}\frac{\partial}{\partial z}T) + \frac{\sigma_E}{c} = 0. \tag{11}$$

Further, we assign $k = \frac{2}{3}c$ and

$$\frac{\partial^2}{\partial z^2}\Big(T^{3/2}\Big) + \frac{\sigma_E}{k} = 0. \tag{12}$$

Here, we focus on the simplest case of the constant energy flux per unit volume (case (i)), however, the analysis presented below can be straightforwardly applied to the cases (ii) and (iii).

For $\sigma_E = \lambda_1$, we can rewrite eq. (12) in dimensionless form as

$$\frac{\partial^2}{\partial \tilde{z}^2}\Big(\widetilde{T}^{3/2}(\tilde{z})\Big) + \widetilde{\lambda_1} = 0, \tag{13}$$

where $\widetilde{T}(\tilde{z}) \equiv T(\tilde{z})/T_0$, $\widetilde{\lambda_1} = \lambda_1 L^2/(kT_0^{3/2})$ and $\tilde{z} \in (-1, 1)$. Using corresponding boundary conditions, we obtain for the unconstrained system

$$\widetilde{T}(\tilde{z}) = \Big(-\frac{\widetilde{\lambda_1}}{2}\tilde{z}^2 + \frac{\widetilde{\lambda_1}}{2} + 1\Big)^{2/3}, \tag{14}$$

and for the constrained system with a wall at $\tilde{z}_1 \equiv L_1/L$,

$$\begin{aligned} \widetilde{T}_1(\tilde{z}) &= \Big(-\frac{\widetilde{\lambda_1}}{2}(\tilde{z} + \widetilde{z_1})^2 + \frac{\widetilde{\lambda_1}}{2}(1 - \widetilde{z_1})^2 + 1\Big)^{2/3}, \\ \widetilde{T}_2(\tilde{z}) &= \Big(-\frac{\widetilde{\lambda_1}}{2}(\tilde{z} + \widetilde{z_1})^2 + \frac{\widetilde{\lambda_1}}{2}(1 + \widetilde{z_1})^2 + 1\Big)^{2/3}. \end{aligned} \tag{15}$$

An example of the temperature profile at $\widetilde{\lambda_1} = 0.5$ and $\widetilde{z_1} = 0.2$ is shown in Fig.1.

With the help of the integrals

$$A = \int_{-1}^{1} \frac{1}{T(\tilde{z})} d\tilde{z}, \quad B = \int_{-1}^{-\tilde{z}_1} \frac{1}{T_1(\tilde{z})} d\tilde{z}, \quad C = \int_{-\tilde{z}_1}^{1} \frac{1}{T_2(\tilde{z})} d\tilde{z}, \tag{16}$$

the energy of the constrained and the unconstrained system is calculated as

$$\widetilde{\varepsilon} = \frac{2}{A}, \quad \widetilde{\varepsilon_1} = \frac{1 - \tilde{z}_1}{B}, \quad \widetilde{\varepsilon_2} = \frac{1 + \tilde{z}_1}{C}. \tag{17}$$

The integrals $A, B$ and $C$ are hypergeometric functions, but we calculate them numerically. The total energy flux is $J_U = \lambda_1 \mathcal{A} 2L$, where $2L$ is the size of the unconstrained system. We have

$$F_0 = \frac{\Delta U}{J_U} = \frac{\varepsilon_0}{\lambda_1}(\widetilde{\varepsilon} - 1), \tag{18}$$

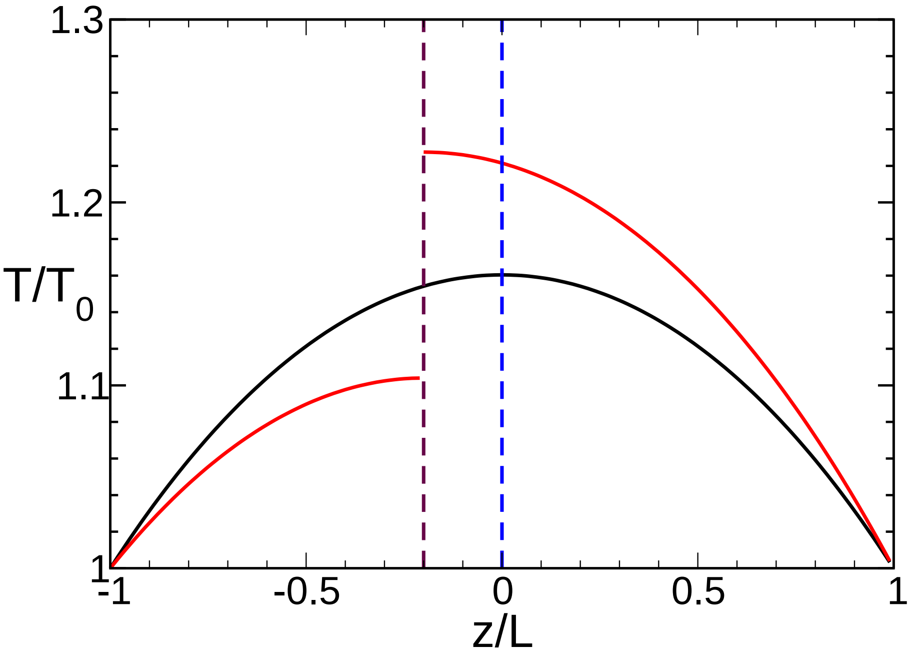


FIG. 1. Normalized temperature profile $\widetilde{T}(\tilde{z})$ for constrained and unconstrained system. Energy supply $\sigma_E = \widetilde{\lambda_1} = 0.5$ and the wall is inserted at $\widetilde{z_1} = 0.2$. The black curve is the temperature profile of the unconstrained system. The blue curves are the temperature profiles of the constrained system. The dashed brown line denotes the position of the wall.

$$F_{1|2} = \frac{U_1 + U_2 - U_0}{J_{U_1} + J_{U_2}} = \frac{\varepsilon_0}{2\lambda_1}(\widetilde{\varepsilon}_1(1 - \tilde{z}_1) + \widetilde{\varepsilon}_2(1 + \tilde{z}_1) - 2). \tag{19}$$

For a given $\lambda_1$, we compare $F_0$ and $F_{1|2}$ by plotting $2\lambda_1(F_{1|2}(\widetilde{z_1}) - F_0)/\varepsilon_0$ (to get rid of unwanted constants) as a function of $\widetilde{z_1}$. For $\lambda_1 = 0.5$ and 15, the results are shown in Fig.2. In these two cases, $\Delta F \geq 0$.

*The simulations in the Lennard-Jones system* Molecular Dynamics (MD) simulations were performed for the system of fixed number $N = 266240$ of the Lennard-Jones (LJ) atoms with the interaction potential truncated and shifted up to make the potential zero at distance $r = 2.5\sigma$ where $\sigma$ is the molecular size parameter in LJ interaction potential [2]. The simulations were

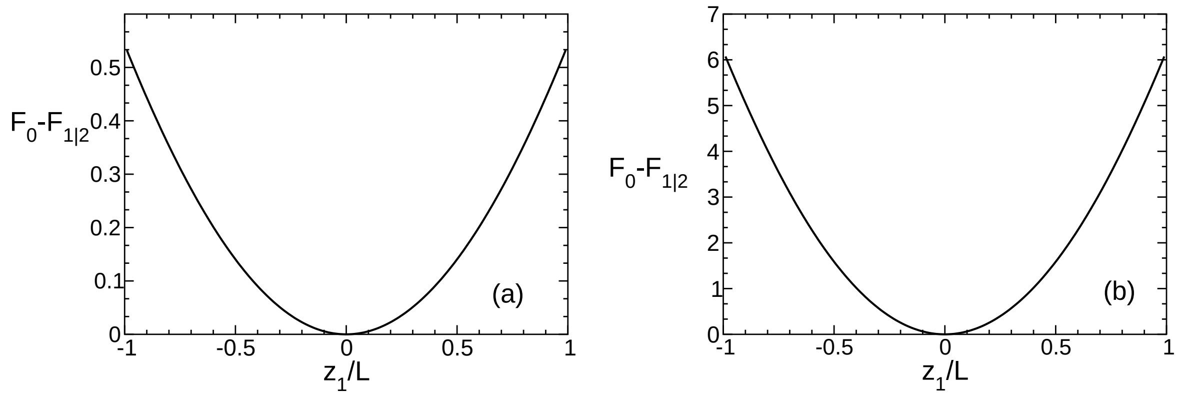


FIG. 2. Difference between $F$ of the constrained and the unconstrained system plotted against wall positions $\widetilde{z}_1$ for $\widetilde{\lambda}_1 = 0.5$ (a) and 15 (b).

performed in the rectangular box of fixed size. The periodic boundary conditions were applied only along the $x, y$ edges of the length $L_x = L_y = 35.22\sigma$ (see Fig. 1 in the main text). The edge along the $z$ direction of constant length $2L = 281.76\sigma$ was restricted by two rigid walls. Two internal walls were added inside the simulation box with the distance between them equal to $\Delta = 4.4\sigma$. This distance guaranteed that atoms at two sides of the double wall would not interact. The LJ atoms interacted with the walls via smooth repulsive potential. The boundary temperature, $T_0 = 0.8\epsilon/k_B$ ($\epsilon$ is the energy parameter in the LJ potential) was kept constant by scaling the absolute value of particle velocities in a close proximity to the walls at $z < b_0$ and $z > 2L - b_0$ where $b_0 = 2.2\sigma$. The simulations were performed for different $L_1$ and $L_2$ such that $L_1 + L_2 + \Delta + 2b_0 = 2L = 281.76\sigma$ was always constant. The mean density of the liquid between the walls $\rho_{mean} = N/((2L - \Delta)L_xL_y) = 0.75\sigma^{-3}$. The Newton equations of motion were solved applying Verlet method [3, 4] with the time step $\delta t = 0.01\sigma(m/\epsilon)^{0.5}$ where $m$ and $\epsilon$ are the particle mass and the LJ energy parameter. The temperature is given in the LJ reduced units where $\epsilon/k_B = 1$ set the temperature scale. The interaction potential between LJ particles and the walls is given by

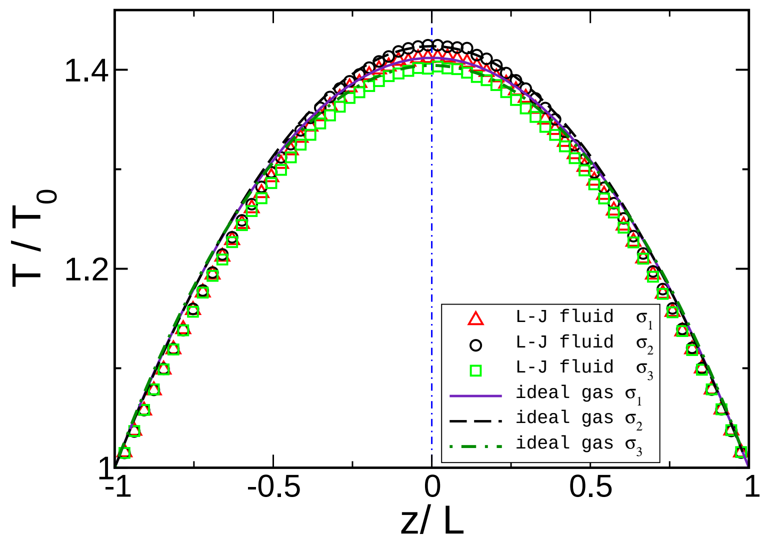


FIG. 3. Scaled stationary temperature profiles for three forms of the source term describing different ways of the energy supply: (i) $\sigma_\varepsilon = \lambda_1$, (ii) $\sigma_\varepsilon = \lambda_2 T(z)$, and (iii) $\sigma_\varepsilon = \lambda_3 \rho(z)$. Symbols show the MD simulations data for the Lennard-Jones system. Lines correspond to the analytical results for an ideal gas with coefficients $\lambda_j$, $j = 1, 2, 3$ chosen to match the MD simulation data at the maximum at $\tilde{z} = z/L = 0$.

$u_B = (z - z_0)^2 \Theta(s(z - z_0))$, where $\Theta$ is the Heaviside theta function and $z_0 = 0$ for left side wall and $L$ for right side wall. Here we present also the figures obtained from the simulations. In Fig 3 we show the temperature profiles in the unconstrained sytem for three modes of the energy transfer with comparison to the temperature profile obtained for the ideal gas by analytical calculations.

*The Rayleigh Benard convection in the 2D system of hard discs (HD)*

Here we will define the simulation parameters. The length of the simulation was measured both in the number of collisions, $n_c$, and in the dimensionless time, $t^*$, defined as follows: $t^* = \frac{t}{t_0}$, where $t_0 = \sqrt{m\sigma^2/(k_B T)}$.

- $g^* = g\frac{mL_y\sigma}{k_B T} = 0.15$

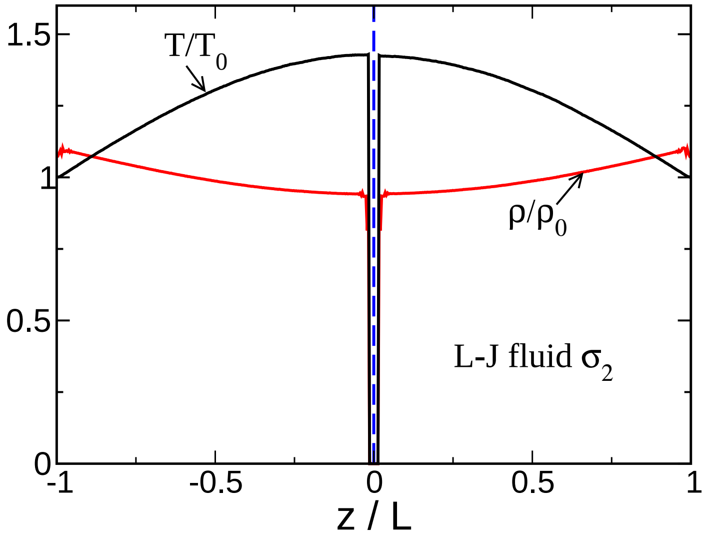


FIG. 4. Scaled stationary temperature and density profiles for $\sigma_\epsilon = \lambda_1$ for a system of LJ particles divided in the middle by the double-wall. The temperature profile has a maximum in the middle of the system, where the density has a minimum. The relation between the profiles comes from the constant pressure in the stationary state $p(\rho(z), T(z)) = const$.

- $N = 10000$ (the $100 \times 200$ box) or $N = 5000$ (the $50 \times 200$ box)
- $n_c = 9 \times 10^8$ collisions for equilibrating and $n_c = 9 \times 10^8$ collisions to calculate the MD averages.
- In case of the $100 \times 200$ box, $n_c = 9 \times 10^8$ corresponds to $t^* = 1.35 \times 10^4$ for $T^* = 10$, and to $t^* = 1.1 \times 10^4$ for $T^* = 25$.

The total energy of the system is calculated as follows:

$$U_{tot} = \sum_{i=1}^{N} \frac{mv_i^2}{2} + \sum_{i=1}^{N} mgy_i \tag{20}$$

where $_i$ is the velocity and $y_i$ is the $y$-coordinate of the $i^{th}$ disk. For $T^* = 1$ the the system reaches

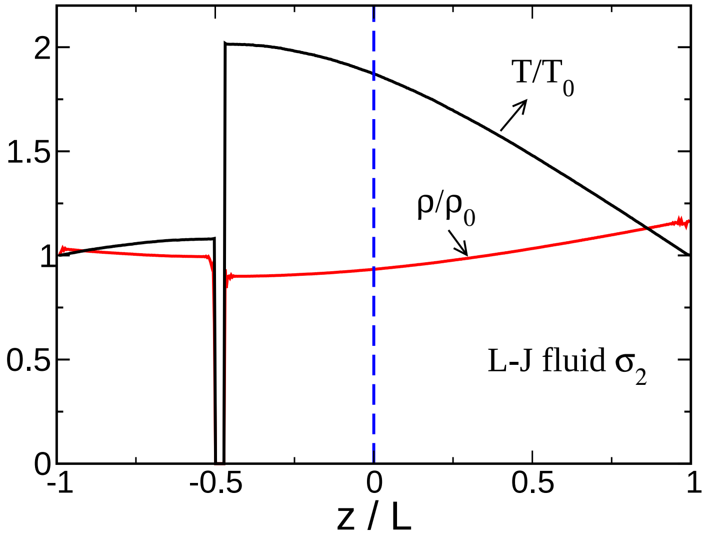


FIG. 5. The same profiles as in Fig. 4, but for unequal partition of the system into two subsystems.

the thermal equilibrium state with an average energy $U_0$. This state serves here as the reference state. For $T^* > 1$ the energy is being pumped into the system at the bottom plate until the system reaches a steady state which can be characterized by the energy stored in the system, $\Delta U$, calculated as $U = U - U_0$, expressed in a dimensionless units as $\Delta U^* = \Delta U/(k_B T)$. For $T^* > 1$ we also determine the energy flow through the upper and lower plates by considering the energy transfer for every single collision of a disk with a plate. In particular, for a single collision, $\alpha$, involving a disk $i$, the energy transfer, $E_\alpha$, is:

$$E_\alpha = \frac{mv^2_{i,after}}{2} - \frac{mv^2_{i,before}}{2} \qquad (21)$$

where $v_{i,before}$ is the the velocity before the collision, and $v_{i,after}$ after the collision.

The energy flux through the upper plate is:

$$J_{upper} = \frac{1}{t} \sum_{\alpha=1}^{n_{c,upper}} E_\alpha \qquad (22)$$

where the summation runs over all disk collisions with the upper plate.

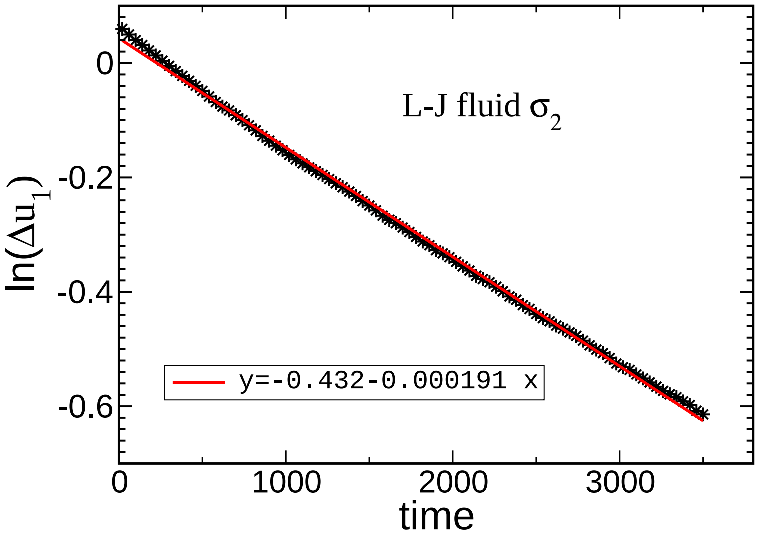


FIG. 6. The change of stored energy $\Delta u_1$ for one particle (for sub-system (1)) as a function of time, t, after shut-down of the energy flux into the system. The energy decreases as $\exp(-t/\tau)$ with the initial decay time $\tau = 2\Delta U_1/J_{U_1}$, where $\Delta U_1$ is the energy stored in the sub-system (1) over its equilibrium value and $J_{U_1}$ is the energy flux in the stationary state, just before the shut-down. The factor 2 comes from the fact that energy flows-out from the system via one wall only.

Similarly, the energy flux through the lower plate is:

$$J_{lower} = \frac{1}{t} \sum_{\alpha=1}^{n_{c,lower}} E_\alpha \tag{23}$$

where the summation runs over all disk collisions with the lower plate. In the stationary state $J_{upper} = -J_{lower}$ Therefore we can use a single dimensionless flux

$$J_U^* = J_{lower} \frac{t_0}{k_B T} \tag{24}$$

which is positive.

[1] R. Livi and P. Politi, *Nonequilibrium Statistical Physics: A Modern Perspective* (Cambridge University Press, Cambridge, 2017).

[2] R.Holyst and M. Litniewski, Phys.Rev.Lett. **100**, 055701 (2008).

[3] M.P. Allen and D.J. Tildesley, *Computer Simulations of Liquids* (Clarendon, Oxford, 1987).

[4] L. Verlet, Phys. Rev. **159**, 98 (1967).
